# Supplementary material for: Probing the Need for Visual Context in Multimodal Machine Translation
Source: arXiv:1903.08678 source file (2019-06-02)
Supplement: Supplementary file 1 [file appendix.tex]

% \subsection{Text Preprocessing}
% The preprocessing pipeline consists of lowercasing, punctuation normalization and tokenization (with aggressive hyphen splitting), all performed using scripts provided by Moses \cite{Moses:2007:acl}. We stitch back the aggressively splitted hyphens prior to computation of all metrics.

% \subsection{Image Preprocessing}
% Prior to feature extraction, we center and standardize the images using ImageNet statistics, resize the shortest edge to 256 pixels and take a center crop of size 256x256. 

% \subsection{Training}
% We use ADAM \cite{kingma2014adam} optimizer with a learning rate of $4e\mathrm{-}4$ and we clip the gradients \cite{pascanu2013difficulty} if the total norm exceeds one. We set the mini-batch size to 64 throughout the experiments. The training is early-stopped if METEOR for \I{dev} set does not improve for ten consecutive epochs. Also, the learning rate is halved whenever the model stops improving for three consecutive epochs. We apply weight decay regularization with a factor of $1e\mathrm{-}5$ over the parameters except the biases. The final hypotheses are decoded using beam search with a beam size of 12.

% \subsection{Model Hyperparameters}
% The encoder and the decoder layers both have 400 hidden units and their initial hidden state is always initialized to 0 except the multimodal system INIT.
% The embedding dimensionality is set to 200. Input and output embeddings on decoder side are tied \cite{press2016using}. A dropout \cite{srivastava2014dropout} of $p=0.4$ and $p=0.5$ is applied on source embeddings and on encoder/decoder outputs, respectively.

% \subsection{Qualitative Examples}
% We provide several qualitative translation examples for color deprivation (Table~\ref{tbl:app_color}), entity masking (Table~\ref{tbl:app_entity}) and progressive masking (Table~\ref{tbl:app_pro}). Comparative multimodal attention maps are also provided for entity masking experiments in Figure~\ref{fig:app_att_1} and \ref{fig:app_att_2}.

% One table of 5 examples per each experiment
%\input{tbl_appendix_examples.tex}
